# Supplementary material for: Robust Anomaly Detection and Backdoor Attack Detection Via Differential Privacy
Source: arXiv:1911.07116 source file (2019-11-16)
Supplement: Supplementary file 1 [file additional-results.tex]

\subsection{Additional experiment results}
We list additional experimental results in this section. With more parameters being tested and more metrics being collected, these extensive results further validate our observations presented in the main paper body: differential privacy could improve anomaly detection and backdoor attack detection; and the higher ratio of outliers in the training data, the more noise (smaller privacy bound $\epsilon$) is needed to achieve the best improvement.

\subsubsection{Autoencoder anomaly detection}
Besides the AUPR scores presented in Table \ref{table:train_ae} for outlier detection and novelty detection using autoencoders, we present additional results with more parameters being tested in Table~\ref{table:ae_appdx_aupr}.
The observations are similar. As an intermediate step in differential privacy to bound the sensitivity, clipping itself without adding any noise is able to improve the performance of outlier detection and novelty detection. Adding various amounts of random Gaussian noise is able to further improve the utility, except when the amount of noise is too big (e.g., $\sigma=50$ and $100$) to ruin the model.
We also indicate the privacy bound $\epsilon$ as accumulated by the moments accountant mechanism in \cite{abadi2016deep}. Interestingly, many $\epsilon$ values are too big to provide any meaningful privacy guarantee, but they are still able to improve the anomaly detection performance.

\begin{table}[hpbt]
	\centering
	\small
	\tabcolsep=0.11cm
    \begin{tabular}{ |l||r|r||r|r||r|r||r|r||r|r||r|r||r| } \hline
    noise   &  \multicolumn{12}{|c|}{outlier percentage in training data $r_o$} & \multirow{3}{*}{$\epsilon$}  \\  \cline{2-13}
    scale    &  \multicolumn{2}{|c||}{$0.01\%$} & \multicolumn{2}{|c||}{$0.1\%$} & \multicolumn{2}{|c||}{$0.5 \%$} & \multicolumn{2}{|c||}{$1\%$} & \multicolumn{2}{|c||}{$5 \%$} & \multicolumn{2}{|c||}{$10\%$}  &   \\ \cline{2-13}
    $\sigma=$ & OD & ND & OD & ND & OD & ND & OD & ND & OD & ND & OD & ND & \\ \hline
     N/A  &  100 & 99.84 & 99.92 & 99.77 & 92.12 & 98.81 & 92.12 & 99.81 & 84.33 & 88.18 & 72.16 & 68.14 & $\infty$    \\ \hline
$0$ & 100 & 99.86 & 99.89 & 99.83 & 98.3 & 99.69 & 95.2 & 98.68 & 83.86 & 87.91 & 77.8 & 74.74 & $\infty$
 \\ \hline
    $0.001$  &  100&99.70  &
100 & 99.86 & 98.37 & 99.64 & 94.33 & 98.81 & 84.31 & 89.34 & 86.51 & 85.58 & $ 1.0\times 10^{10}$
 \\ \hline
    $  0.005$  & 100 & 99.87 & 99.82 & 99.78  & 98.69 & 99.7 & 95.67 & 98.87 & 91.01 & 94.3 & 79.55 & 77.04 & 
$3.9\times 10^8$
 \\ \hline
    $  0.01$  &  {\bf 100} & {\bf 99.89} & {\bf 100} & {\bf 99.97} &94.92 & 99.23  &97.08 & 99.33  &90.79 & 93.34  &85.41 & 84.07 & $9.8 \times 10^7$
 \\ \hline

    $  0.05$  &  100 & 99.85 & 99.89 & 99.79 & 97.97 & 99.55   &
96.94 & 99.34 & 88.84 & 92.54 & 75.18 & 72.09 & $2.8 \times 10^6 $
 \\ \hline

    $  0.1$  & 100 & 99.88 & 100 & 99.85 &
{\bf 98.44} & {\bf 99.66} &
93.11 & 98.21 &
92.23 & 94.21                     &
85.56 & 83.98 & $6.8 \times 10^4$
 \\ \hline

    $ 0.5$  &  100& 99.84 & 99.95 & 99.85 & 98.59 & 99.64 & {\bf 99.95} & {\bf 99.85} & 93.69 & 95.8 & 85.61 & 83.86 & 22.23
\\ \hline
    $  1$  &  100 & 99.81  &100 & 99.78 &98.28 & 99.67 &95.8 & 99.0   &94.92 & 96.87 &81.87 & 80.12  & 3.09
\\ \hline

    $  5$  &  100 & 99.49 & 99.87 & 99.49 & 98.51 & 99.52 &
96.5 & 98.78   &
{\bf 96.78} & {\bf 98.04} &
95.25 & 95.41 &  0.44
\\ \hline
$ 10$  & 97.62 & 97.61 & 90.24 & 97.77 & 91.88 & 98.2  &97.5 & 99.12  &96.6 & 98.2  & {\bf 97.07} & {\bf 97.46}  &  0.25
\\ \hline
\multicolumn{14}{|c|}{{\sf Below $\sigma$ value is too big such that the model does not converge well in training.}} \\ \hline
$  50$  &  54.19 & 90.46 & 65.94 & 92.13 & 70.34 & 90.8 & 78.34 & 91.19 & 86.58 & 91.59 & 88.49 & 90.27 & 0.19
\\ \hline
$  100$  &  56.08 & 87.2 & 47.22 & 70.57 & 71.95 & 90.8 & 4.23 & 10.73 & 80.58 & 86.94 & 89.26 & 90.68 & 0.19
\\ \hline
    \end{tabular}
\caption{{AUPR scores for autoencoder outlier detection (OD) and novelty detection (ND)}. }
\label{table:ae_appdx_aupr}
\end{table}

Besides AUPR scores, we further present AUROC scores in Table~\ref{table:ae_appdx_auroc} for the same set of experiments. Autoencoders, as validated by many previous works (\cite{mirsky2018kitsune,gottschlich2017autoperf}), present great effectiveness in detecting outliers and novelties, especially when the outlier ratio in training dataset is slow (e.g., below $1\%$). Although not as obvious as AUPR scores, the improvements brought by differential privacy follow a similar trend, where the improvement is more significant with larger noise (smaller $\epsilon$) being applied to models trained with more outliers.

\begin{table}[hpbt]
	\centering
	\small
	\tabcolsep=0.11cm
    \begin{tabular}{ |l||r|r||r|r||r|r||r|r||r|r||r|r||r| } \hline
    noise   &  \multicolumn{12}{|c|}{outlier percentage in training data $r_o$} & \multirow{3}{*}{$\epsilon$}  \\  \cline{2-13}
    scale    &  \multicolumn{2}{|c||}{$0.01\%$} & \multicolumn{2}{|c||}{$0.1\%$} & \multicolumn{2}{|c||}{$0.5 \%$} & \multicolumn{2}{|c||}{$1\%$} & \multicolumn{2}{|c||}{$5 \%$} & \multicolumn{2}{|c||}{$10\%$}  &   \\ \cline{2-13}
    $\sigma=$ & OD & ND & OD & ND & OD & ND & OD & ND & OD & ND & OD & ND & \\ \hline
N/A & 100 & 99.97 & 100 & 99.95 & 99.81 & 99.79 & 99.17 & 99.07 & 97.3 & 97.4 & 89.46 & 89.2 & $\infty$  \\ \hline
0 & 100 & 99.97 & 100 & 99.97 & 99.96 & 99.93 & 99.7 & 99.77 & 97.36 & 97.52 & 92.39 & 92.35 & $\infty$  \\ \hline
0.001 & 100 & 99.93 & 100 & 99.97 & 99.89 & 99.84 & 99.79 & 99.82 & 97.37 & 97.63 & 96.26 & 96.72 & $1.0\times 10^{10}$  \\ \hline
0.005 & 100 & 99.96 & 100 & 99.95 & 99.92 & 96.09 & 99.81 & 99.83 & 98.73 & 98.91 & 93.62 & 93.82 & $3.9\times 10^{8}$  \\ \hline
0.01 & 100 & 99.97 & 100 & 99.97 & 99.8 & 99.87 & 99.89 & 99.9 & 98.39 & 98.5 & 96.02 & 96.4 & $9.8\times 10^{7}$  \\ \hline
0.05 & 100 & 99.97 & 100 & 99.96 & 99.9 & 99.93 & 99.87 & 99.9 & 97.55 & 97.81 & 90.91 & 90.87 & $2.8\times 10^{6}$  \\ \hline
0.1 & 100 & 99.97 & 100 & 99.97 & 99.87 & 99.9 & 99.58 & 99.71 & 98.77 & 98.82 & 96.16 & 96.46 & $6.8\times 10^{4}$  \\ \hline
0.5 & 100 & 99.96 & 100 & 99.97 & 99.9 & 99.91 & 99.77 & 99.85 & 99.13 & 99.25 & 95.96 & 96.25 & 22.23  \\ \hline
1 & 100 & 99.95 & 100 & 99.94 & 99.91 & 99.94 & 99.74 & 99.81 & 99.31 & 99.44 & 94.66 & 94.95 & 3.09  \\ \hline
5 & 100 & 99.81 & 100 & 99.85 & 99.96 & 99.93 & 99.52 & 99.5 & 99.07 & 99.32 & 98.49 & 98.74 & 0.44  \\ \hline
10 & 100 & 99 & 99.86 & 99.25 & 99.14 & 99.93 & 99.68 & 99.79 & 98.72 & 99.29 & 98.9 & 99.27 & 0.25  \\ \hline
\multicolumn{14}{|c|}{{\sf Below $\sigma$ value is too big such that the model does not converge well in training.}} \\ \hline
50 & 99.99 & 96.11 & 94.8 & 96.41 & 92.96 & 96.13 & 94.15 & 96.29 & 7.03 & 5.95 & 93.83 & 95.61 & 0.19  \\ \hline
100 & 99.73 & 94.7 & 82.64 & 87.29 & 93.51 & 99.22 & 31.77 & 30.91 & 94.47 & 96.08 & 94.62 & 96.09 & 0.19  \\ \hline
    \end{tabular}
\caption{{AUROC scores for autoencoder outlier detection (OD) and novelty detection (ND)}. }
\label{table:ae_appdx_auroc}
\end{table}

\subsubsection{Improvements over DeepLog}
To compare the differentially private models with DeepLog, we utilize the same anomaly detection criteria, i.e., Top-\textit{k} based anomaly detection as what's presented in \cite{du2017deeplog}. Nevertheless, as a direct extension of the idea in measuring model loss for anomaly detection, we also tested the classification probability as one type of threshold for anomaly detection. 
In particular, if an actual system log entry is predicted with a probability lower than some threshold $T_p$, we treat this log entry as a detected anomaly.
While the baseline DeepLog results are not as good as the Top-\textit{k} based detection, we show that similarly, differential privacy is able to significantly reduce the number of false negatives, without introducing too many new false positives.

\Paragraph{Probability-based detection.}
As a preliminary result, we use probability-based anomaly detection to demonstrate the effectiveness of differential privacy noise in reducing \fn. Table~\ref{table:prob} shows \fn and \fp for DeepLog and DeepLog+DP with increasing noise levels, under different probability thresholds $T_p$. It is clear that differential privacy noise could effectively reduce \fn, and the larger noise being added, the more false negatives are reduced. We also note that when $\sigma=0.25$, the privacy bound $\epsilon=90.5$. It is often thought that a privacy bound $\epsilon>20$ is completely useless in terms of protecting privacy. Here we indicate that a small amount of noise may be enough to reduce \fn. Although more false positives are incurred because of differential privacy noise, the drop in \tpr is negligible, considering the large volume of normal data. For example, when $T_p=2 \times 10^{-6}$ and $\sigma=1$, the \fn drop from 1261 to 183 indicates a \tnr increase of 8\% ($91.7\% \to 98.8\%$), while the \fp increase from 2291 to 3734 only shows a \tpr decrease of 0.3\% ($99.59\% \to 99.32\%$).

\begin{table}[hbt]
% \vspace{-1mm}
	\centering
	\small
    \begin{tabular}{ |l|r|r|r|r|r| } \hline
    Probability & {DeepLog}  &  \multicolumn{4}{|c|}{DeepLog+DP (\fn/\fp)}  \\  \cline{3-6}
    threshold {$T_p$}    & \fn/\fp & $\sigma=0.25$ & $\sigma=1$ & $\sigma=1.5$ & $\sigma=2$   \\ \hline
%    $1e-4$  & 89/5855 &  1/19614 & 0/13672 & 0/25080  &  1/22967   \\ \hline
    $10^{-5}$  &   573/3596  &  7/14268 & 0/6059 &1/8213   &   1/9187   \\ \hline
    $2\times 10^{-6}$  &  1261/2291 & 208/4756  & 183/3734 &1/5718   &  1/6317 \\ \hline
    $10^{-6}$  &  1468/2068 & 410/3759 & 190/3552 & 2/4002   &  1/6093 \\ \hline
    \end{tabular}
	\caption{{Probability-based anomaly detection results}. }
	\label{table:prob}
\end{table}

\begin{table*}[htb]
	\centering
	\tabcolsep=0.12cm
    \begin{tabular}{ |l|r|r|r|r|r|r|r|r|r| } \hline
     & \multirow{ 2}{*}{DeepLog}  &  \multicolumn{8}{|c|}{DeepLog+DP}  \\  \cline{3-10}
     &  & $\sigma$=$0.25$ & $\sigma$=$0.5$ & $\sigma$=$0.75$ & $\sigma$=$1.0$ & $\sigma$=$1.25$ & $\sigma$=$1.5$ & $\sigma$=$1.75$  & $\sigma$=$2.0$   \\ \hline
    AUROC score & 0.9993   & 0.9997  & 0.9997 & 0.9997  & 0.9998 & 0.9993  & 0.9994 & 0.9989 & 0.9985 \\ \hline
    privacy bound $\epsilon$ & 0  & 90.45  & 6.21 & 1.86   &  0.96 & 0.61 & 0.42 & 0.31 & 0.25 \\ \hline
    \end{tabular}
	\caption{{AUROC score comparison and privacy bound $\epsilon$}. }
	\label{table:auc}
\end{table*}

\paragraph{AUROC score}
To evaluate the overall performance of DeepLog+DP compared with DeepLog under different thresholds,
we further compute the AUROC score of DeepLog and DeepLog+DP with different noise scale $\sigma$.
% \auc stands for \textit{Area under curve (\auc) score}, which is the area under 
% \textit{receiver operating characteristic (ROC) curve}, where the x axis is the \fpr while the y axis denotes the \tpr. Clearly, the lower the \fpr and the higher the \tpr, the bigger the area under ROC curve, and hence the larger the \auc score.
As shown in Table~\ref{table:auc}, DeepLog already achieves excellent AUROC score, considering the large amount of normal data and the significantly fewer anomalies. However, an adequate amount of differential privacy noise is still able to improve the performance. 

\paragraph{Privacy bound $\epsilon$}
Table~\ref{table:auc} also indicates the privacy bound $\epsilon$. Note that $\epsilon<10$ is often considered as usable and $\epsilon<1$ is a tight bound that well protects privacy. Considering all the cases, $\sigma=1$ gives the best anomaly detection utility as well as a tight privacy bound to protect training data privacy.

\subsubsection{Backdoor attack detection}
In this section, we evaluate more parameters for the experiment set up described in Section~\ref{sec:exp-backdoor} {BACKDOOR ATTACK DETECTION}, and measure  \textit{benign accuracy}, \textit{success rate}, AUPR score and AUROC score as explained in Section~\ref{sec:exp-backdoor} for each experiment setting.
Similar as the observations in Section~\ref{sec:exp-backdoor}, a differentially private trained machine learning model is naturally more robust to backdoor attacks. The evidence is that the benign accuracy (Table \ref{table:train_bk_benign_appdx}) is affected little by differential privacy except when the noise scale is too big to ruin the model parameters, compared with the significant downgrade (e.g., 98.1\% to 0.3\%) in backdoor success rate (Table \ref{table:train_bk_success_appdx}). Also, as shown in Table \ref{table:bk_aupr_appdx} and Table \ref{table:bk_auroc_appdx}, measuring model loss to detect poisoning examples could be useful when the poisoning ratio is low. Nevertheless, applying differential privacy is able to significantly improve the detection performance for a poisoning ratio as high as $45\%$.

\begin{table}[hpbt]
	\centering
	\small
    \begin{tabular}{ |l|r|r|r|r|r|r|r|r|r| } \hline
   noise scale  & \multicolumn{8}{c|}{poisoning ratio in training data $r_p$} & \multirow{2}{*}{$\epsilon$} \\ \cline{2-9}
   $\sigma$ & 0.005 & 0.01 & 0.05 & 0.1 & 0.2 & 0.3 & 0.4 & 0.45 &   \\ \hline
N/A & 98.93 & 99.03 & 98.95 & 99.11 & 98.94 & 99.06 & 99.05 & 98.97 & $\infty$  \\ \hline
0 & 97.66 & 97.21 & 97.84 & 97.46 & 96.97 & 96.32 & 93.61 & 92.4 & $\infty$ \\ \hline
0.001 & 97.5 & 97.52 & 97.72 & 97.29 & 97.47 & 96.69 & 94.16 & 90.41 & $9.9\times 10^{9}$ \\ \hline
0.005 & 97.57 & 97.55 & 97.46 & 97.75 & 97.36 & 96.5 & 93.96 & 91.25 & $3.9\times 10^{8}$ \\ \hline
0.01 & 97.51 & 97.61 & 97.4 & 97.55 & 97.27 & 97.07 & 94.77 & 92.82 & $9.8\times 10^{7}$ \\ \hline
0.05 & 97.42 & 97.87 & 97.8 & 97.72 & 97.69 & 96.37 & 94.19 & 93.28 & 2830766.11 \\ \hline
0.1 & 97.55 & 97.84 & 97.7 & 97.34 & 97.29 & 96.91 & 94.11 & 91.36 & 67915.88 \\ \hline
0.5 & 97.56 & 97.29 & 97.28 & 97.37 & 97.13 & 96.55 & 95.19 & 86.37 & 22.23 \\ \hline
1 & 96.94 & 96.95 & 96.96 & 96.53 & 96.27 & 95.78 & 91.65 & 83.16 & 3.09 \\ \hline
2 & 93.76 & 93.39 & 92.16 & 93.22 & 92.77 & 92.4 & 87.61 & 81.24 & 1.18 \\ \hline
\multicolumn{10}{|c|}{{\sf Below noise level $\sigma$ could be too high.}} \\ \hline
3 & 89.85 & 89.5 & 91.12 & 90.92 & 89.35 & 89.81 & 85.42 & 76.51 & 0.75 \\ \hline
5 & 80.51 & 79.57 & 80.49 & 80.28 & 79.19 & 77.95 & 57.5 & 61.64 & 0.44 \\ \hline
10 & 17.32 & 19.82 & 20.31 & 12.07 & 11.34 & 11.43 & 11.15 & 11.11 & 0.25 \\ \hline
\end{tabular}
\caption{{Benign accuracy of models trained on datasets with different poisoning ratio $r_p$. The more noise being added, the more utility is affected.}}
\label{table:train_bk_benign_appdx}
\end{table}

\begin{table}[hpbt]
	\centering
	\small
    \begin{tabular}{ |l|r|r|r|r|r|r|r|r|r| } \hline
   noise scale  & \multicolumn{8}{c|}{poisoning ratio in training data $r_p$} & \multirow{2}{*}{$\epsilon$} \\ \cline{2-9}
   $\sigma$ & 0.005 & 0.01 & 0.05 & 0.1 & 0.2 & 0.3 & 0.4 & 0.45 &   \\ \hline
N/A & 47.85 & 90.96 & 97.12 & 98.1 & 98.46 & 98.91 & 98.92 & 98.79 & $\infty$ \\ \hline
0 & 0.23 & 0.29 & 0.35 & 0.3 & 0.47 & 0.74 & 68.1 & 72.02 & $\infty$ \\ \hline
0.001 & 0.21 & 0.22 & 0.25 & 0.37 & 0.42 & 0.85 & 35.83 & 19.01 & $9.9\times 10^{9}$ \\ \hline
0.005 & 0.17 & 0.2 & 0.28 & 0.3 & 0.35 & 35.54 & 50.28 & 83.94 &  $3.9\times 10^{8}$ \\ \hline
0.01 & 0.25 & 0.24 & 0.34 & 0.31 & 0.42 & 0.56 & 93.64 & 15.25 & $9.8\times 10^{7}$ \\ \hline
0.05 & 0.24 & 0.25 & 0.37 & 0.3 & 0.37 & 18.55 & 82.15 & 4.53 & 2830766.11 \\ \hline
0.1 & 0.25 & 0.18 & 0.28 & 0.39 & 0.47 & 0.71 & 82.23 & 59.57 & 67915.88 \\ \hline
0.5 & 0.26 & 0.23 & 0.29 & 0.35 & 0.37 & 0.81 & 1.63 & 74.15 &  22.23 \\ \hline
1 & 0.28 & 0.3 & 0.45 & 0.5 & 0.63 & 1.09 & 44.12 & 67.44 & 3.09 \\ \hline
2 & 0.74 & 0.68 & 1.07 & 1.1 & 1.4 & 2.67 & 5.95 & 71.48 & 1.18 \\ \hline
\multicolumn{10}{|c|}{{\sf Below noise level $\sigma$ could be too high.}} \\ \hline
3 & 0.96 & 1.22 & 1.1 & 1.59 & 2.69 & 2.66 & 6.02 & 20.38 & 0.75 \\ \hline
5 & 2.01 & 1.6 & 2.44 & 3.47 & 2.68 & 8.15 & 13.78 & 19.91 & 0.44 \\ \hline
10 & 9.93 & 10.3 & 10.03 & 9.08 & 9.68 & 9.33 & 10.14 & 9.77 & 0.25 \\ \hline
\end{tabular}
\caption{{Backdoor attack success rate of models trained on datasets with different poisoning ratio $r_p$. The success rate is significantly reduced for models trained with differential privacy.}}
\label{table:train_bk_success_appdx}
\end{table}

\begin{table}[hpbt]
	\centering
	\small
    \begin{tabular}{ |l|r|r|r|r|r|r|r|r|r| } \hline
   noise scale  & \multicolumn{8}{c|}{poisoning ratio in training data $r_p$} & \multirow{2}{*}{$\epsilon$} \\ \cline{2-9}
   $\sigma$ & 0.005 & 0.01 & 0.05 & 0.1 & 0.2 & 0.3 & 0.4 & 0.45 &  \\ \hline
N/A & 73.01 & 27.02 & 14.85 & 17.63 & 24.9 & 36.42 & 42.16 & 45.85 & $\infty$ \\ \hline
0 & 91.22 & 92.11 & 95.33 & 95.46 & 95.9 & 96.55 & 62.57 & 60.33 & $\infty$  \\ \hline
0.001 & 91.52 & 93.36 & 94.61 & 95.98 & 96.95 & 96.05 & 78.53 & 86.9 & $9.9\times 10^{9}$ \\ \hline
0.005 & 92.64 & 94.04 & 94.76 & 95.45 & 96.98 & 79.1 & 72.73 & 52.07  & $3.9\times 10^{8}$ \\ \hline
0.01 & 92.24 & 94.03 & 93.4 & 95.76 & 96.69 & 96.22 & 47.08 & 90.77  & $9.8\times 10^{7}$ \\ \hline
0.05 & 90.76 & 95.11 & 95.09 & 95.54 & 96.35 & 87.28 & 49.82 & 93.72  & 2830766.11 \\ \hline
0.1 & 92.16 & 94.85 & 95.33 & 95.28 & 96.4 & 96.67 & 51 & 65.9  & 67915.9 \\ \hline
0.5 & 92.76 & 93.4 & 94.5 & 94.93 & 95.74 & 95.88 & 95.96 & 54.99  &  22.23 \\ \hline
1 & 88.67 & 90.31 & 94.77 & 94.46 & 96.03 & 94.67 & 72.99 & 56.35  & 3.09 \\ \hline
2 & 65.01 & 78.51 & 80.76 & 87.54 & 88.76 & 87.63 & 86.75 & 51.41  & 1.18 \\ \hline
\multicolumn{10}{|c|}{{\sf Below noise level $\sigma$ could be too high.}} \\ \hline
3 & 29.31 & 51.37 & 78.25 & 81 & 79.83 & 81.56 & 84.46 & 71.62  & 0.75 \\ \hline
5 & 6.4 & 17.39 & 58.66 & 58.88 & 61.8 & 69.19 & 64.27 & 61.58  & 0.44 \\ \hline
10 & 0.8 & 2 & 10.12 & 10.88 & 20.32 & 30.89 & 40.92 & 45.17  & 0.25 \\ \hline
\end{tabular}
\caption{{AUPR scores for backdoor attack detection. Applying differential privacy significantly improves the results.}}
\label{table:bk_aupr_appdx}
\end{table}

\begin{table}[htbp]
	\centering
	\small
    \begin{tabular}{ |l|r|r|r|r|r|r|r|r|r| } \hline
   noise scale  & \multicolumn{8}{c|}{poisoning ratio in training data $r_p$} & \multirow{2}{*}{$\epsilon$} \\ \cline{2-9}
   $\sigma$ & 0.005 & 0.01 & 0.05 & 0.1 & 0.2 & 0.3 & 0.4 & 0.45 &  \\ \hline

N/A&99.26&95.23&78.88&67.72&59.47&60.9&55.33&52.73& $\infty$  \\ \hline
0&99.92 & 99.88&99.79 & 99.72&99.51 & 99.31&70.24 & 62.88 & $\infty$ 	\\ \hline
0.001&99.91 & 99.88&99.79 & 99.72&99.62 & 99.27&81.27 & 88.1 & $9.9\times 10^{9}$  \\ \hline
0.005&99.9 & 99.93&99.79 & 99.75&99.63 & 84.51&75.12 & 60.21 & $3.9\times 10^{8}$  \\ \hline
0.01&99.92 & 99.92&99.74 & 99.74&99.61 & 99.3&61.83 & 93.78& $9.8\times 10^{7}$  \\ \hline
0.05 & 99.9 & 99.94&99.83 & 99.73&99.59 & 90.67&58.03 & 97.12 & 2830766.11  \\ \hline
0.1&99.93 & 99.93&99.82 & 99.69&99.55 & 99.37&59.71 & 65.55 & 67915.88  \\ \hline
0.5&99.95 & 99.92&99.76 & 99.68&99.5 & 99.23&98.68 & 58.44 &   22.23 \\ \hline
1&99.86 & 99.84&99.76 & 99.61&99.43 & 98.87&75.7 & 63.94&3.09 \\ \hline
2&99.64 & 99.64&98.97 & 98.86&98.21 & 97.13 & 94.82 & 57.81&1.18  \\ \hline
\multicolumn{10}{|c|}{{\sf Below noise level $\sigma$ could be too high.}} \\ \hline
3&98.68 & 98.92&98.68 & 98.17&96.73 & 95.92&93.86 & 81.22&0.75 \\ \hline
5&95.74 & 96.13&96.38 & 94.42&92.22 & 89.52&77.77 & 73.11&0.44  \\ \hline
10&56.77 & 60.49&61.2 & 53.11&51.05 & 51.33 & 51.19 & 50.35 & 0.25  \\ \hline
\end{tabular}
\caption{{AUROC scores for backdoor attack detection. It shows that measuring model loss for poisoning samples detection could be effective when the poisoning ratio is low. Differential privacy improves the performance in all cases, except when the noise scale is too big to ruin the model parameters.}}
\label{table:bk_auroc_appdx}
\end{table}
